# Supplementary material for: LISA: Learning-Integrated Space Partitioning Framework for Traffic Accident Forecasting on Heterogeneous Spatiotemporal Data
Source: arXiv:2412.15365 source file (2024-12-19)
Supplement: Supplementary file 1 [file 8.Appendix.tex]

\section{Appendix}

\noindent\textbf{Feature Summary:} Our framework deals with three types of input features: spatial, temporal, and spatiotemporal. In this work, we extract 47 features as the input, including 5 temporal features(e.g., day of year, holiday), 29 spatial features (e.g., total road length, avg. speed limit), and 13 spatiotemporal features (e.g., traffic volume) for each location $l$ and time interval $t$. SpatialGraph features are generated spectral features\cite{yuan2018hetero}. Details are shown in Table. \ref{table: feature}

\begin{table}[ht]
	\centering
	%\small
	\caption{Feature Table}
	\scalebox{0.80}{
	\begin{tabular}{|c|c|}
		\hline
    	\textbf{Feature Group} & \textbf{Feature List}\\
		\hline
		\hline
		$F_T$ & \pbox{20cm}{\textbf{5 calendar features:}\\ day of the week, day of the year, month of the year, \\
		whether this is a holiday, whether this is weekend} \\
		\hline
		$F_S$ & \pbox{20cm}{\textbf{13 POI features:}\\ eat-drink, going-out, sights-museums, transport,\\ accommodation, shopping, leisure-outdoor, \\administrative-areas-buildings, natural-geographica,\\ petrol-station, atm-bank-exchange,\\toilet-rest-area, hospital-health-care-facility \\\textbf{6 basic road condition features:}\\ Annual Average Daily Traffic, average speed limit, \\  average mileage for each road, \\number of intersections,\\ the total mileage of road system, \\and total annually traffic volume\\ \textbf{10 SpatialGraph features  \cite{yuan2018hetero}}} \\
		\hline
		$F_{ST}$ & \pbox{20cm}{\textbf{9 weather features:} \\ average air temperature, highest temperature, \\ lowest temperature, wind speed, precipitation, \\ snowfall, snow depth, dew point temperature,\\ and MERRA\\ \textbf{4 real-time traffic condition features:} \\ average traffic speed, normal vehicle traffic volume, \\ truck traffic volume, and Occupancy}\\

		\hline

	\end{tabular}
	\label{Features}
	}
\end{table}

\textbf{Performance across Partitions} We investigate how the proposed model performs at each partition. The problem is that we cannot compare the model errors between different partitions directly, because model errors in the urban area are likely to be greater than the model error in a rural area since there are frequent accidents in the urban area daily. Therefore, lower error in the rural area does not necessarily indicate better performance of the model. To solve this issue, we use the Historical Average as a reference value to measure the overall improvements of our proposed work at each partition, since we want to examine if LISA can capture those complex accident patterns. We calculate the percent of improvements between our proposed method and the historical average across partitions. 

\begin{figure}[ht]  \hspace*{0cm}
 \centering
 \includegraphics[width = 0.45\textwidth]{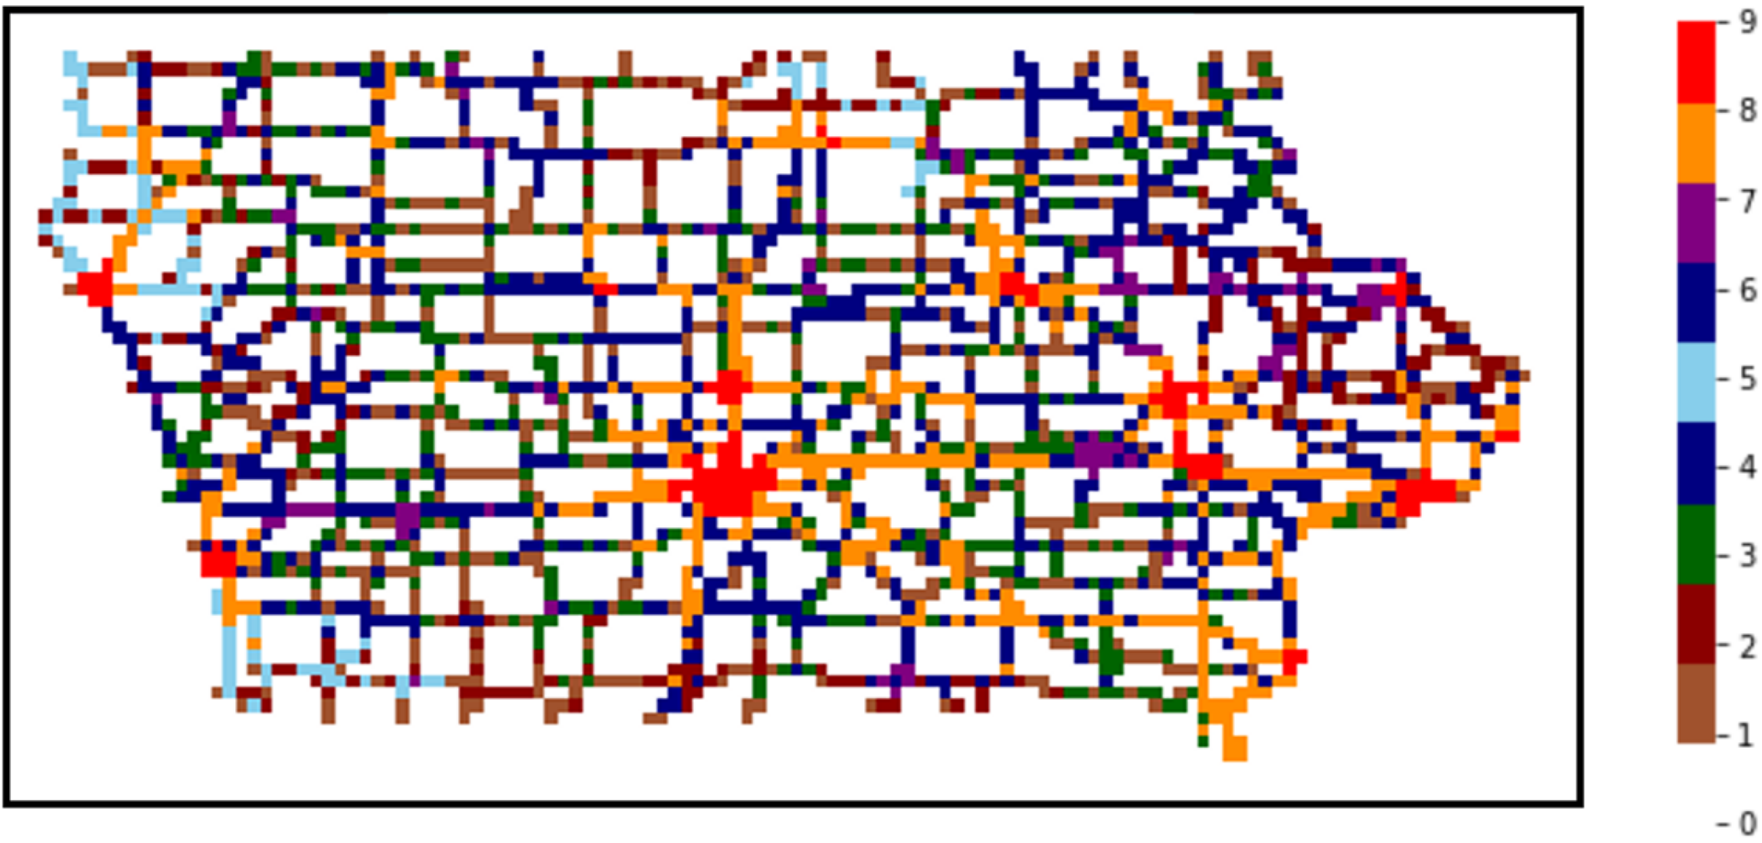}
 \caption{Spatial partitions of the study area learned by LISA (Colors indicate different partitions and numbers indicate the order of acquiring partitions)}
 \label{fig: partition}
\end{figure}

Figure \ref{fig: partition} shows the partitioned study area, and nine partitions are represented by different colors in the figure. The bar chart in Figure \ref{fig: trend} demonstrates the improvements in percentage from partition 1 to partition 9. As can be observed, from the most rural area to the most urban area, it appears a slight upward trend and achieves an average of $28\%$ improvements on most partitions.

\begin{figure}[ht] \hspace*{0cm}
 \centering
 \includegraphics[width = 0.42\textwidth]{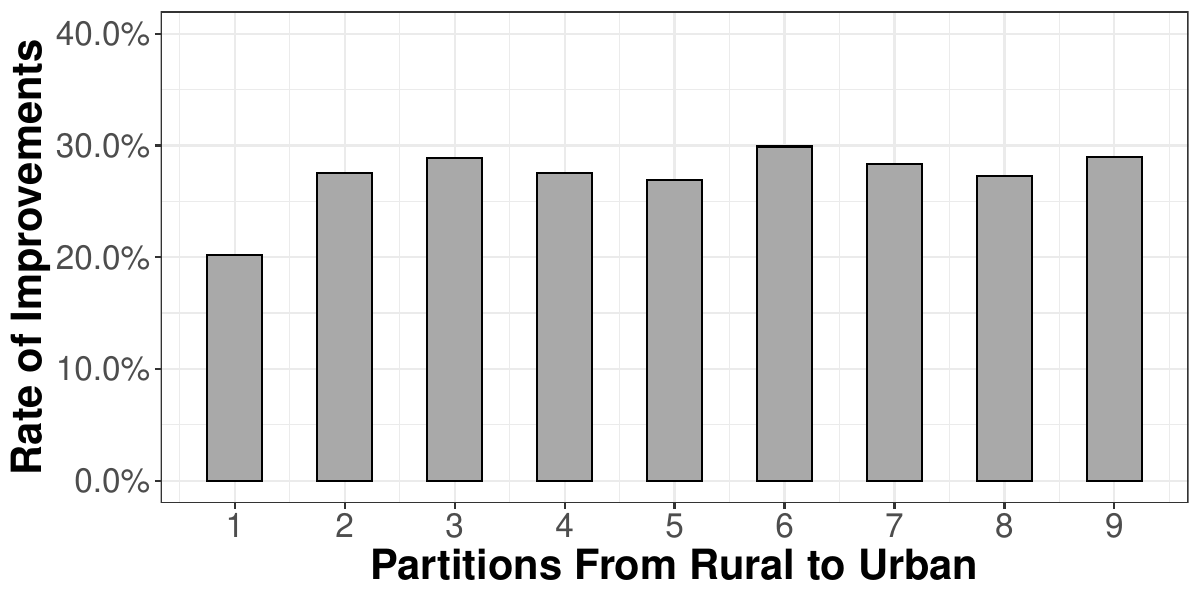}
 \caption{Performance improvements compared with HA across learned partitions}
 \label{fig: trend}
\end{figure}
